# Supplementary material for: Data Exploration, Quality Control and Testing in Single-Cell qPCR-Based Gene Expression Experiments
Source: arXiv:1210.1226 source file (2012-10-03)
Supplement: Supplementary file 1 [file supplement.pdf]

# Supplement to "Data Exploration, Quality Control and Testing in Single-Cell qPCR-Based Gene Expression Experiments"

Andrew McDavid, Greg Finak, Pratip K. Chattopadyay, Maria Dominguez, Laurie Lamoreaux, Steven S. Ma, Mario Roederer and Raphael Gottardo

## 1 Data sets and notations

The empirical cumulative distribution of $\pi$ and $\mu$ for data sets A, B, C is depicted in Supplementary Figure 1. Null wells lower the maximum value of $\pi$ in experiments B and C. After filtering, this difference is no longer noted. Normal quantile-quantile plots of the robust z-transformed $et$ for expressed genes $z_{ij}$ are depicted in Supplementary Figure 4-6. The hypothesized normal distribution fits most genes well.

## 2 Derivation of combined Likelihood Ratio Statistic

Consider the composite, two-sample test:

$$H_0 : \pi_0 = \pi_1 \quad \text{and} \quad \mu_0 = \mu_1$$

versus the alternative

$$H_a : \pi_0 \neq \pi_1 \quad \text{and} \quad \mu_0 \neq \mu_1.$$

between the stimulated and un-stimulated groups. Suppose both groups share a common variance, $\sigma^2$. Omitting the gene index $j$ for clarity, the likelihood ratio test is defined as

$$\Lambda(\mathbf{y}, \mathbf{v}) = \frac{\sup_{\boldsymbol{\theta} \in H_0} \mathrm{L}(\boldsymbol{\theta}|\mathbf{y}, \mathbf{v})}{\sup_{\boldsymbol{\theta} \in H_A} \mathrm{L}(\boldsymbol{\theta}|\mathbf{y}, \mathbf{v})} \tag{1}$$

where the likelihood is given by

$$\mathrm{L}(\boldsymbol{\theta}|\mathbf{y}, \mathbf{v}) = \prod_k \pi_k^{n_k} (1 - \pi_k)^{I - n_k} \prod_{i \in S_k} g(y_{ik}|\mu_k, \sigma^2), \tag{2}$$

$\mathbf{y}$ and $\mathbf{v}$ are the vectors of observations for the gene across the two groups, $\boldsymbol{\theta} = \{\mu_k, \sigma^2, \pi_k; k = 0, 1\}$ is the vector of unknown parameters, $S_k$ is the set of cells expressing the gene in group $k$ (*i.e.* $S_k = \{i : v_{ik} = 1\}$) , $n_k = \sum_i v_{ik}$ is the number of cells expressing the gene in group $k$, and $g$ is the density function of the log-normal distribution with parameters $\mu_k$ and $\sigma^2$. Using the following change of variable, $et_{ik} = \log y_{ik}$, in (3), the likelihood function can be written as

$$\mathrm{L}(\boldsymbol{\theta}|\mathbf{et}, \mathbf{v}) = \prod_k \pi_k^{n_k} (1 - \pi_k)^{I - n_k} \prod_{i \in S_k} \mathrm{N}(et_{ik}|\mu_k, \sigma^2) \tag{3}$$

where $\mathrm{N}(\cdot|\mu, \sigma^2)$ is the density function of a normal distribution with mean $\mu$ and variance $\sigma^2$. It follows that the likelihood ratio test can be written as

$$\begin{aligned}
\Lambda(\mathbf{et}, \mathbf{v}) &= \frac{\sup_{\boldsymbol{\theta} \in H_0} \mathrm{L}(\boldsymbol{\theta}|\mathbf{et}, \mathbf{v})}{\sup_{\boldsymbol{\theta} \in H_A} \mathrm{L}(\boldsymbol{\theta}|\mathbf{et}, \mathbf{v})} \\
&= \frac{\sup_{\{\pi_0, \mu_0, \sigma^2\}} \pi_0^{n_0 + n_1} (1 - \pi_0)^{2I - n_0 - n_1} \prod_k \prod_{i \in S_k} \mathrm{N}(et_{ik}|\mu_0, \sigma^2)}{\sup_{\{\pi_0, \mu_0, \sigma^2, \pi_1, \mu_1\}} \prod_k \pi_k^{n_k} (1 - \pi_k)^{I - n_k} \prod_{i \in S_k} \mathrm{N}(et_{ik}|\mu_k, \sigma_k^2)} \\
&= \frac{\sup_{\pi_0} \pi_0^{n_0 + n_1} (1 - \pi_0)^{2I - n_0 - n_1}}{\sup_{\{\pi_0, \pi_1\}} \prod_k \pi_k^{n_k} (1 - \pi_k)^{I - n_k}} \cdot \frac{\sup_{\{\mu_0, \sigma^2\}} \prod_k \prod_{i \in S_k} \mathrm{N}(et_{ik}|\mu_0, \sigma^2)}{\sup_{\{\mu_0, \sigma^2, \mu_1\}} \prod_k \prod_{i \in S_k} \mathrm{N}(et_{ik}|\mu_k, \sigma^2)} \\
&= \Lambda_b(\mathbf{v}) \cdot \Lambda_n(\mathbf{et}^+)
\end{aligned}$$

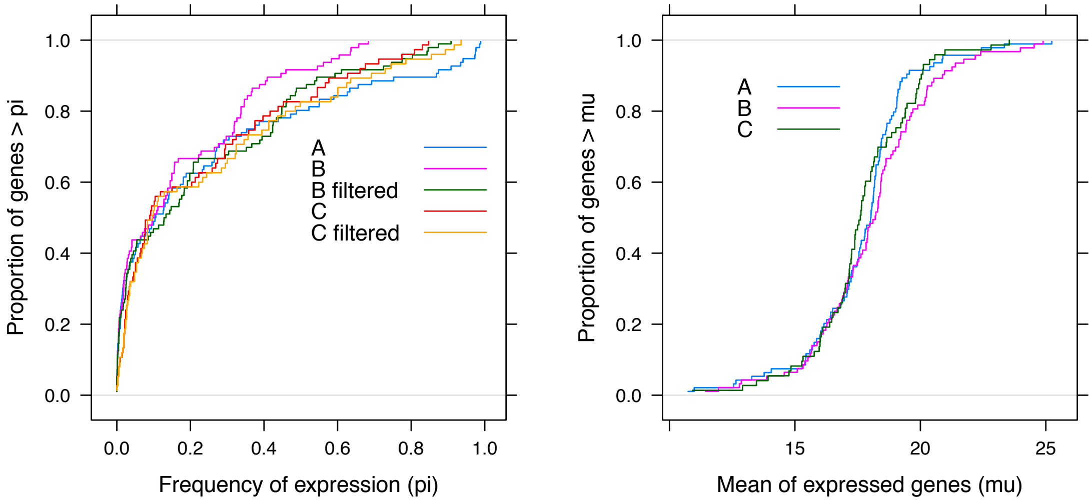


Supplementary Figure 1: Empirical cumulative distribution of $\pi$ and $\mu$ for data sets A, B, C.

where $\Lambda_b$ is a binomial LRT, $\Lambda_n$ is a normal LRT and $\mathbf{et}^+$ is the set of positive et values. Thus our combine LRT can be computed as the product of a binomial and a normal LRTs, both of which can easily be derived using classical statistical theory.

## 3 Filtering Parameter Optimization

We determine appropriate values of the continuous parameter $t_z$ and the expression proportion parameter $t_\zeta$ by searching the grid $t_z, t_\zeta \in [3, 4, \ldots, 9]$.For each value in the grid, the weighted residual sum of squares $\overline{\text{WSS}}$ is calculated. The minimizing values vary somewhat on the data set, so we based our recommendation of $t_z = t_\zeta = 9$by choosing values that minimize the maximum residual $\overline{\text{WSS}}$ across data sets.

Supplementary Figure 2 depicts the hundred-cell/single-cell concordance and $\overline{\text{WSS}}$ for data set A for $t_z = 9, \ldots, 3$ and $t_\zeta = 9, \ldots, 3$.The points depict the position of a gene after filtering at a given stringency. Since there is a natural nesting of the parameters, we consider them cumulatively and allow $t_z$ to vary fastest. Thin lines indicate the position of a gene at the previous filtering stringency. Thus, for example between $(t_z, t_\zeta) = (9, 3)$ and $(t_z, t_\zeta) = (7, 3)$ one additional cell is filtered, so there is one thin, dark line, whereas at $(t_z, t_\zeta) = (5, 3)$, two genes move to the y-axis.

| | | $t_z$ | | | |
|---|---|---|---|---|---|
| Data set | $t_\zeta$ | 3 | 5 | 7 | 9 |
| A | 3 | 6.44 | 2.95 | 2.95 | 2.83 |
| A | 5 | 5.26 | 1.17 | 0.11 | 0.00 |
| A | 7 | 5.26 | 0.01 | 0.40 | 1.02 |
| A | 9 | 5.21 | 0.00 | 0.43 | 1.64 |
| B | 3 | 8.85 | 5.33 | 5.56 | 6.28 |
| B | 5 | 3.18 | 0.00 | 0.04 | 0.69 |
| B | 7 | 3.18 | 0.00 | 0.04 | 0.69 |
| B | 9 | 3.18 | 0.00 | 0.04 | 0.69 |
| C | 3 | 27.99 | 16.88 | 8.56 | 8.56 |
| C | 5 | 27.98 | 8.90 | 7.08 | 6.13 |
| C | 7 | 25.84 | 6.41 | 4.55 | 0.00 |
| C | 9 | 25.84 | 6.41 | 4.55 | 0.00 |

Supplementary Table 1: $\overline{\text{WSS}} - \min_{t_z, t_\zeta, \text{noutlier}} \overline{\text{WSS}}$ values across data sets and filtering parameters. For each data set, the minimum $\overline{\text{WSS}}$ is subtracted so that cells that achieve that value contain zeroes.

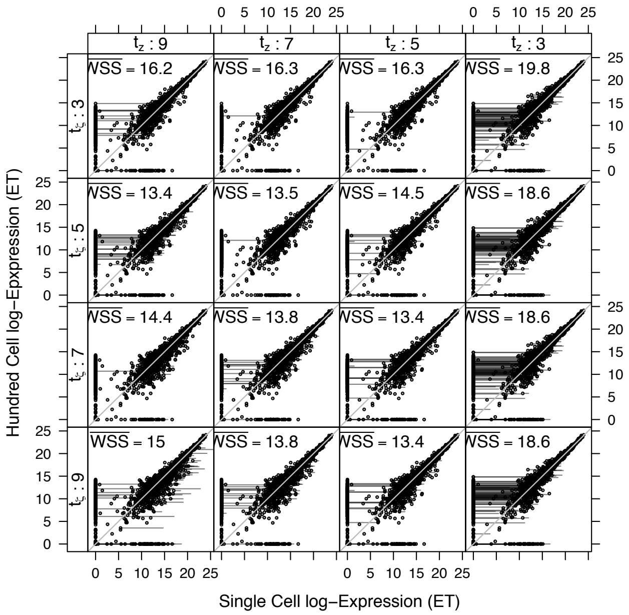


Supplementary Figure 2: Hundred cell-single cell concordance as filtering stringency increases from bottom left to upper right; data set A.

Supplementary Table 1 shows the $\overline{\text{WSS}}$ in all three data sets for all points in the grid described above.

# 4 Filtering and housekeeping genes

Scatter plots and linear fits (Supplementary Figure 3) between housekeeping genes and other frequently expressed genes suggest filtering suffices to remove technical artifacts, so normalization is unnecessary.

Outlying and high-leverage points–most of which are flagged for filtering–drive most of the apparent correlation between genes, since there is very little trend in the central portion of the distribution.

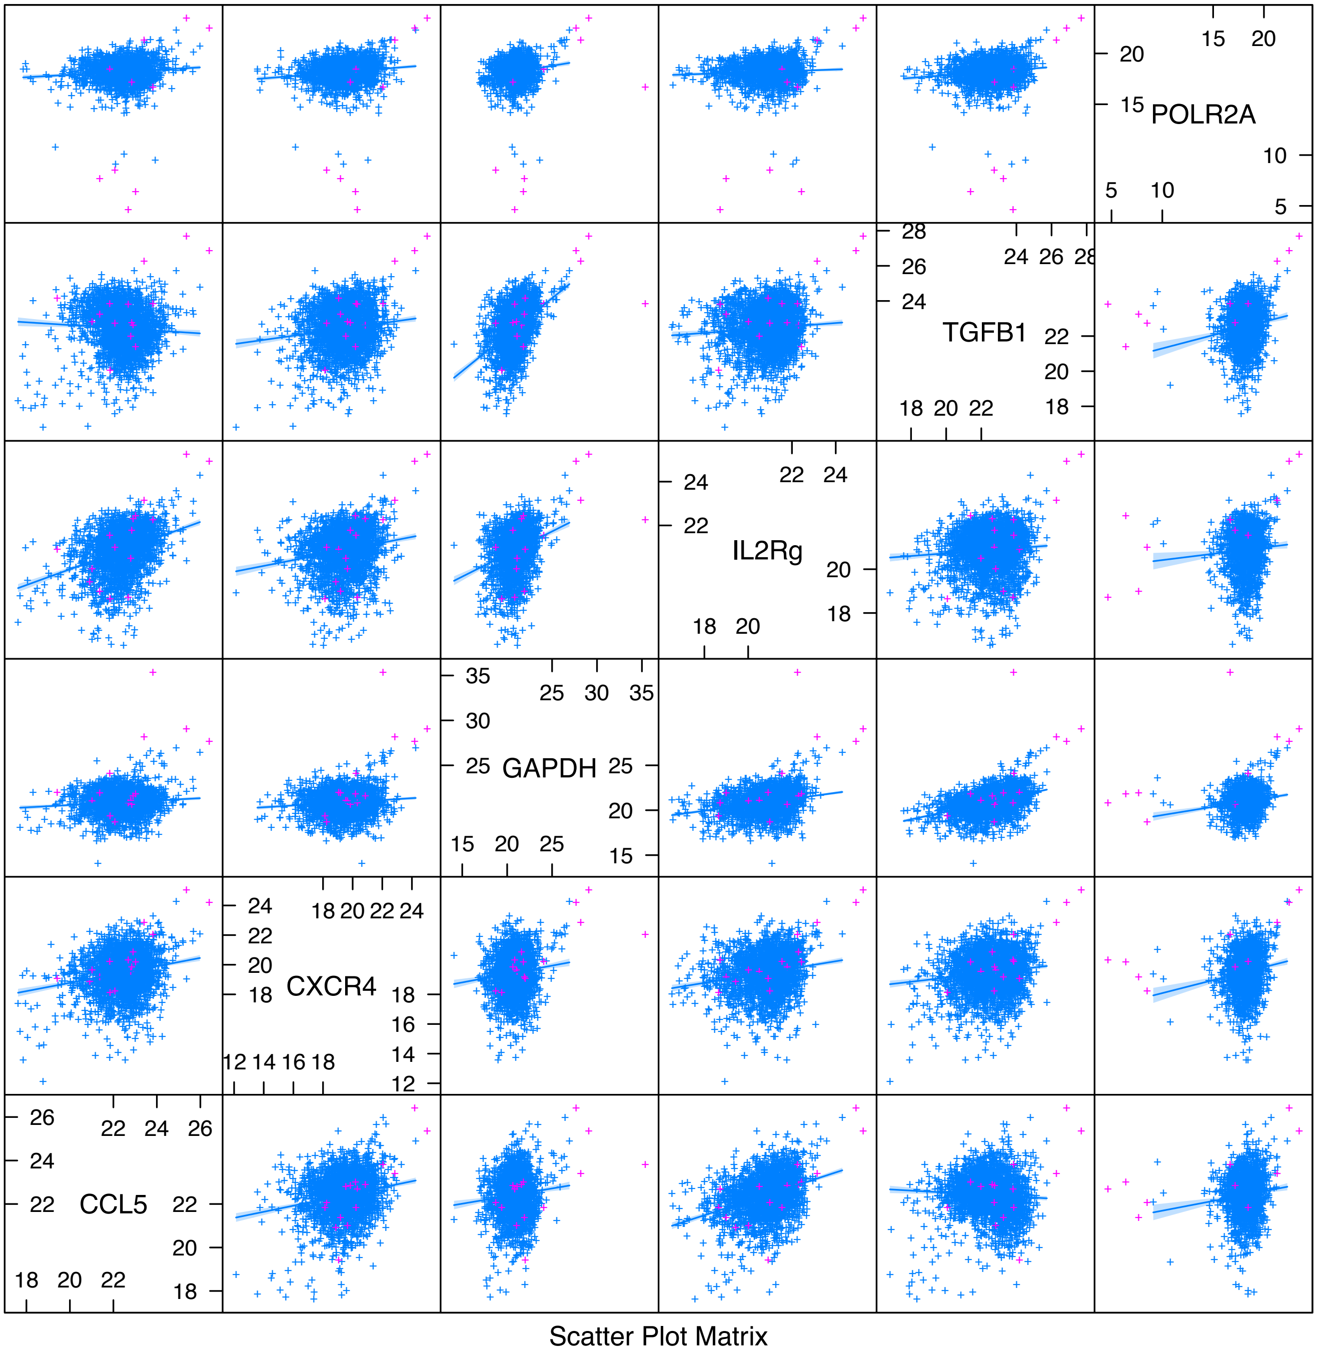


Supplementary Figure 3: Scatter plots of housekeeping genes GAPDH, POLR2A and other frequently expressed ($\pi > .95$) genes. Cells flagged for filtering are indicated in purple. A regression line of the form $et_y \sim et_x + \text{intercept}$, and its standard error is plotted using unfiltered cells.

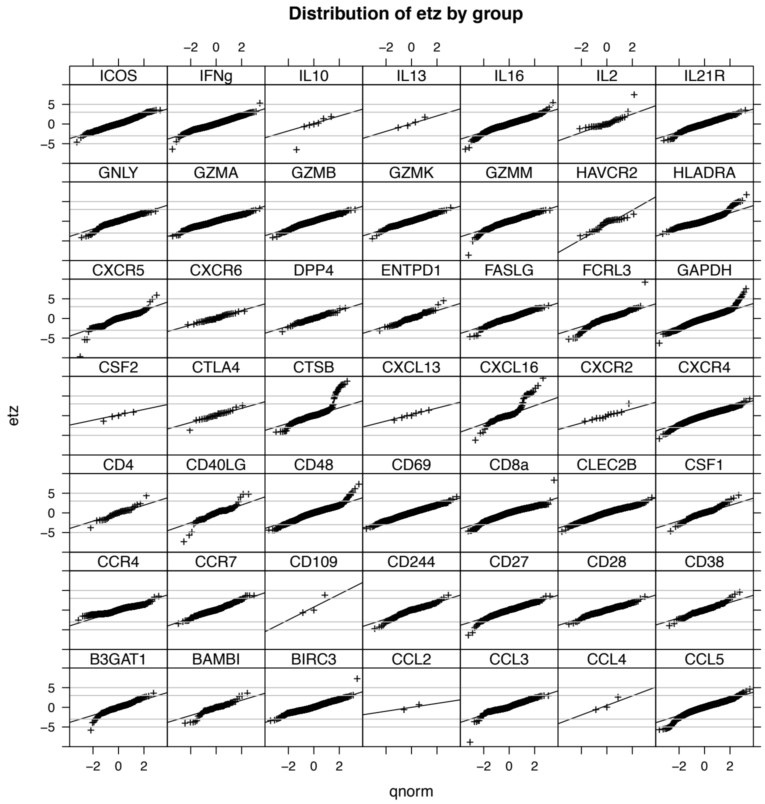


Supplementary Figure 4: Normal quantile-quantile plots of $z_{ij}$ for 49 genes, data set A.

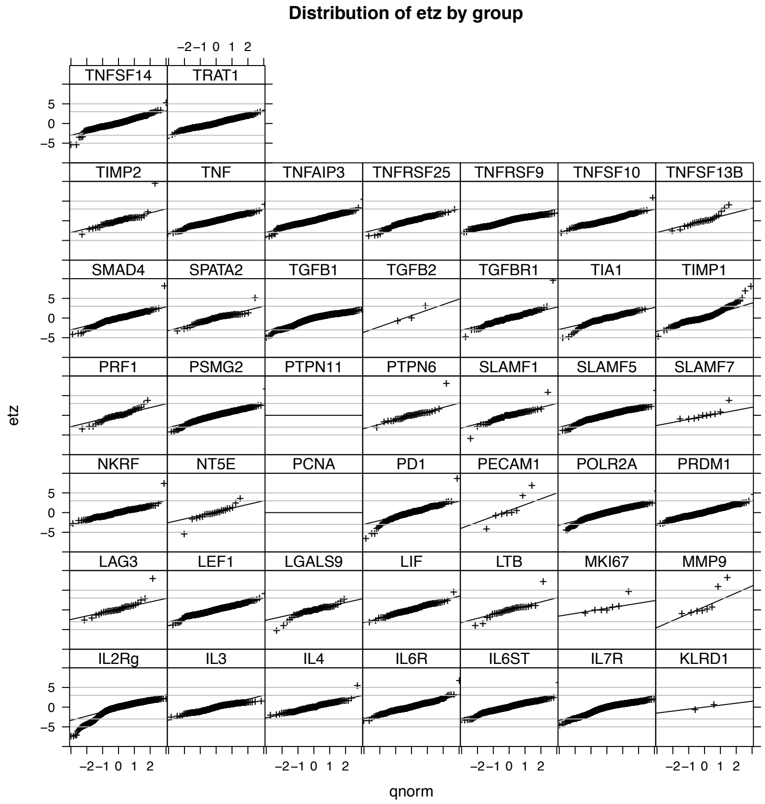


Supplementary Figure 5: Normal quantile-quantile plots of $z_{ij}$ for 44 genes, data set B.

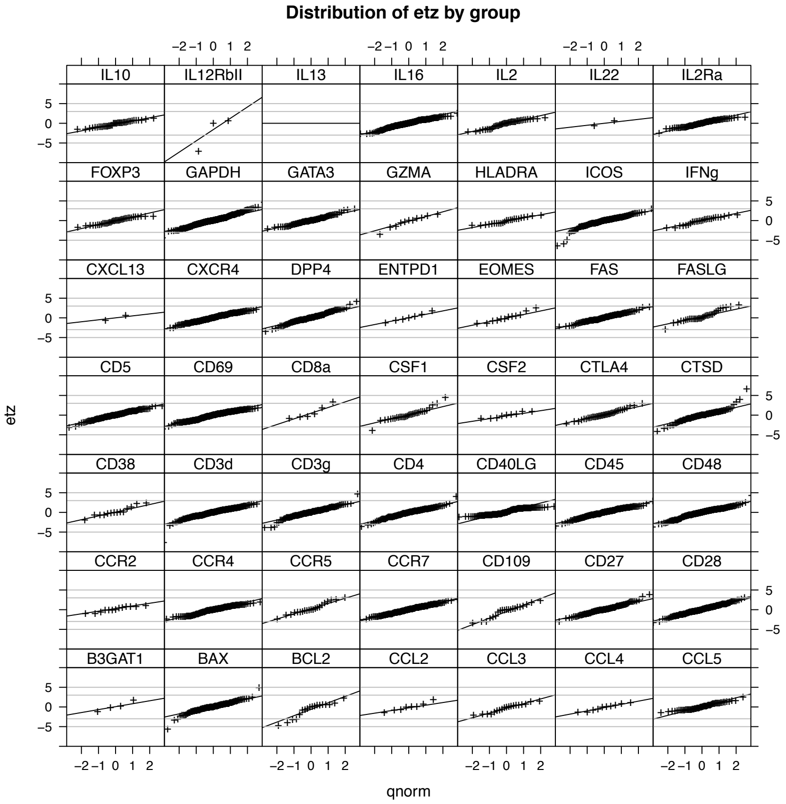


Supplementary Figure 6: Normal quantile-quantile plots of $z_{ij}$ for 49 genes, data set C.
